# Supplementary material for: Marangoni swimmer pushing particle raft under 1D confinement
Source: arXiv:2508.15205 ancillary file (2025-08-21)
Supplement: Supplementary file 1 [file Supplementary_information.pdf]

# Supplementary information for Marangoni swimmer pushing particle raft under 1D confinement

Abhradeep Maitra[1], Anupam Pandey[2], Sebastien Michelin[3], Sunghwan Jung[4]

[1] *Department of Mechanical and Aerospace Engineering, Cornell University, Ithaca, NY 14853, USA*

[2] *Mechanical and Aerospace Engineering, Syracuse University, Syracuse, USA*

[3] *LadHyX – Ecole Polytechnique, Palaiseau, France*

[4] *Department of Biological and Environmental Engineering, Cornell University, Ithaca, NY 14853, USA*

### A. Contact angle of passive particles at the air-water interface

The contact angle ($\theta_{\mathrm{p}}$) of the hollow glass microspheres (passive particles) was measured using a direct imaging method. A small amount of particles was introduced at the air-water interface of a circular polystyrene Petri dish (diameter = 36 mm) filled with deionized water. The floating particles were imaged using a zoom lens (Navitar 1-60135 6.5X Zoom with 12mm Fine Focus along with a 1.5x lens attachment, NAVITAR 1-60112 and a 2x adapter, NAVITAR 1-6030) on a DSLR camera (NIKON). The particles were imaged with an inclined view to specifically capture the portion of the particles above the air-water interface (see setup in Fig. S1a). Using image analysis, the contact angle was estimated for the particles by first fitting a circle to the particle's outline and then measuring the angle between the tangent to the particle surface at the meniscus and the horizontal (representing the interface, see Fig. S1b). It was assumed that the interface is almost flat near the particle. The results of the contact angle measurement are plotted as a distribution in Fig. S1c. The contact angle was calculated to be $102° \pm 9.8°$. Also, the radius of the fitted circle was used to estimate the particle radius ($r_{\mathrm{p}}$, Fig. S2).

## I. VIDEOS

**Movie S1.** Video of a swimmer performing uni-directional motion at a nearly constant speed in an annular channel without passive particles at the interface. The plots show the temporal evolution of swimmer speed ($v_{\mathrm{s}}$) and azimuthal position in the channel ($\alpha$), respectively.

**Movie S2.** Steady uni-directional motion of swimmer in annular channel for three different initial packing fraction of particles i.e. $\phi_{\mathrm{ini}} = 0.04$, 0.16 and 0.44. The plots show the temporal evolution of swimmer speed ($v_{\mathrm{s}}$) and azimuthal position in the channel ($\alpha$), respectively.

**Movie S3.** Oscillatory motion of swimmer in annular channel for initial packing fraction $\phi_{\mathrm{ini}} \approx 0.64$. The plots show the temporal evolution of swimmer speed ($v_{\mathrm{s}}$) and azimuthal position in the channel ($\alpha$), respectively.

**Movie S4.** Sporadic motion of swimmer in annular channel for initial packing fraction $\phi_{\mathrm{ini}} \approx 0.82$. The plots show the temporal evolution of swimmer speed ($v_{\mathrm{s}}$) and azimuthal position in the channel ($\alpha$), respectively.

**Movie S5.** Velocity vectors (blue arrows) from PIV analysis, representing the local velocity of particles being pushed by the swimmer in the annular channel, for a representative experiment.

**Movie S6.** Video showing a magnified view of swimmer pushing a particle raft in an annular channel, utilized for measuring the packing fraction in the raft.

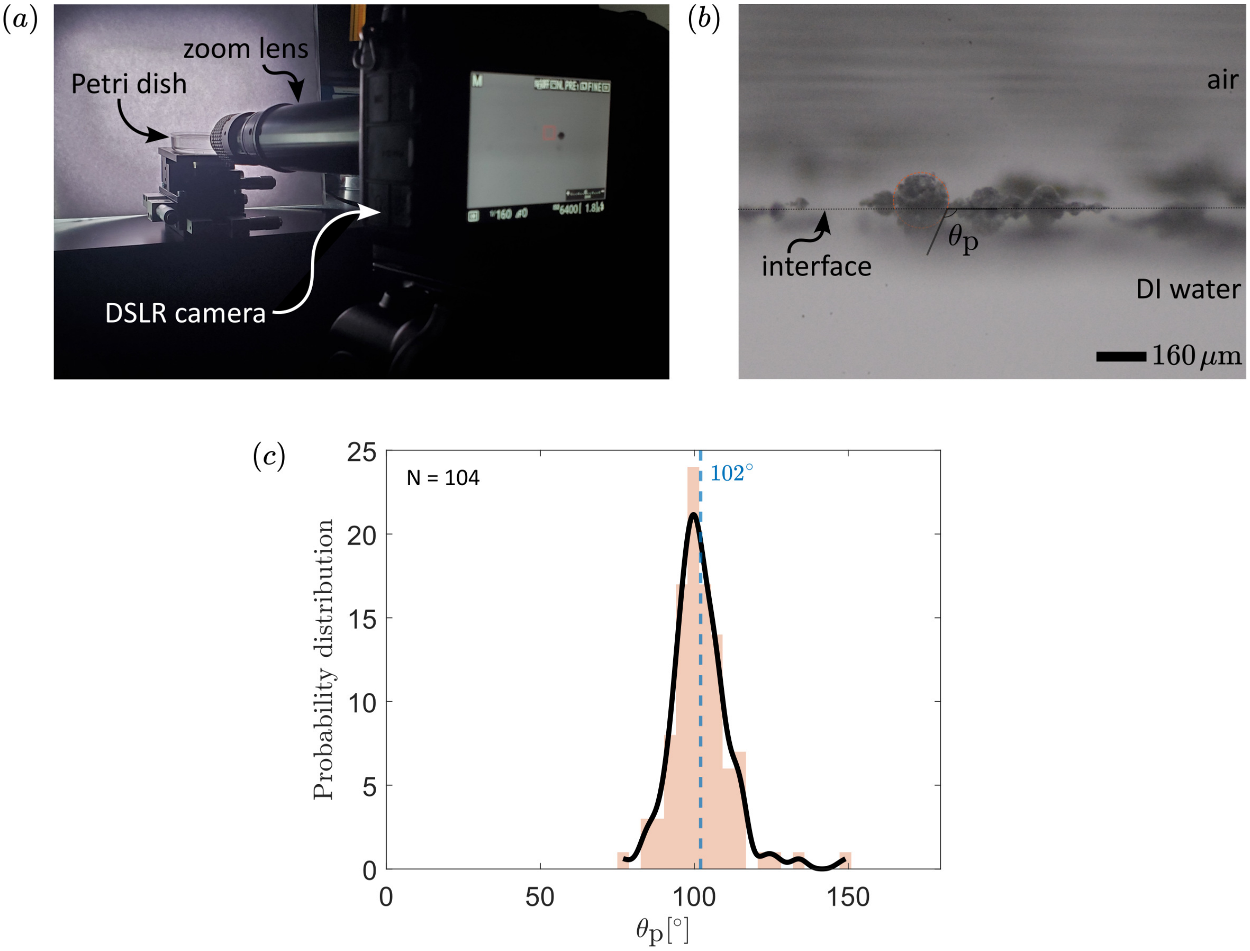


FIG. S1. (a) Experimental setup for direct imaging of particle contact angle. (b) Representative snapshot of hollow glass microspheres floating at the air-water interface, used for measuring contact angle. The dotted horizontal line represents the interface. Above the dotted line is air while below it is DI water. The dotted orange arc around one of the particles represents the fitted circle. (c) Distribution of the measured contact angle $\theta_\mathrm{p}$. The contact angle for the hollow glass microspheres was estimated to be $102° \pm 9.8°$ based on a sample size (N) of 104 particles.

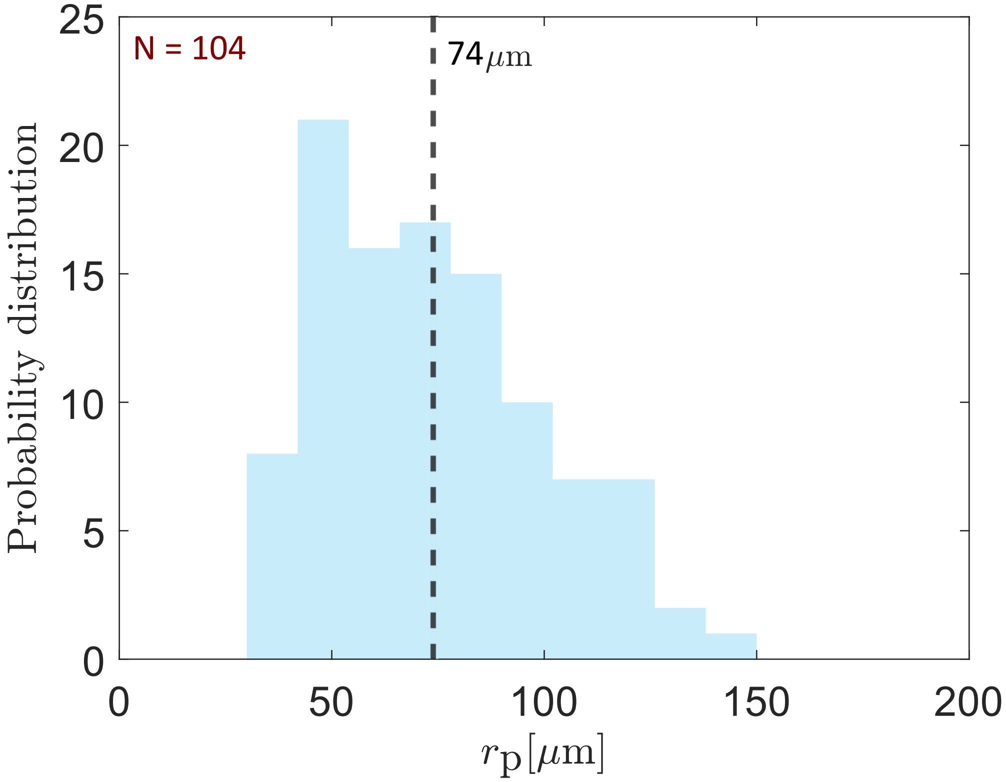


FIG. S2. (a) Distribution of the passive particle radius $r_{\rm p}$ measured from images of the particles floating at air-water interface. The radius of the hollow glass microspheres was estimated to be 74±26 $\mu$m based on a sample size (N) of 104 particles.

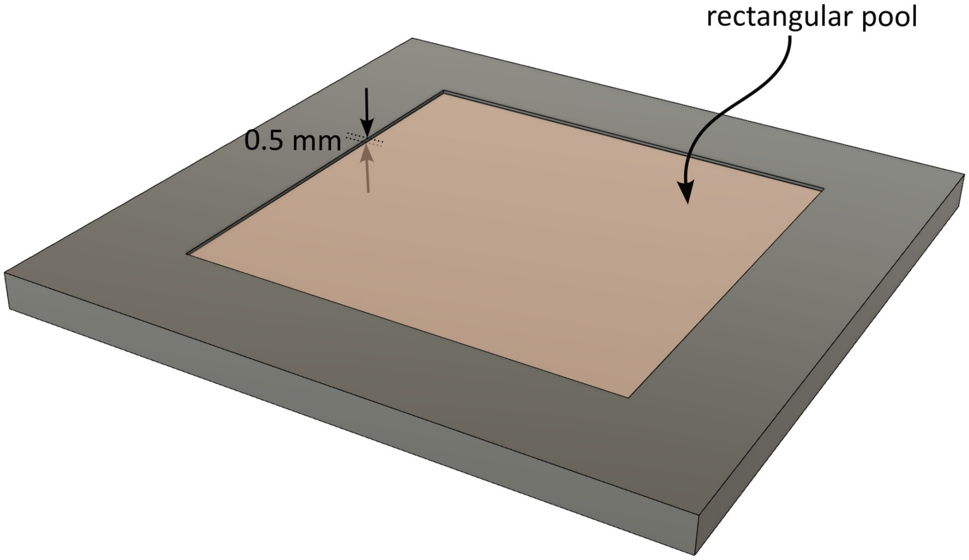


FIG. S3. (a) A schematic of the SLA printed part used to prepare the agar gel sheet of 0.5 mm thickness. The shaded brown portion is the pool with a depth of 0.5 mm.

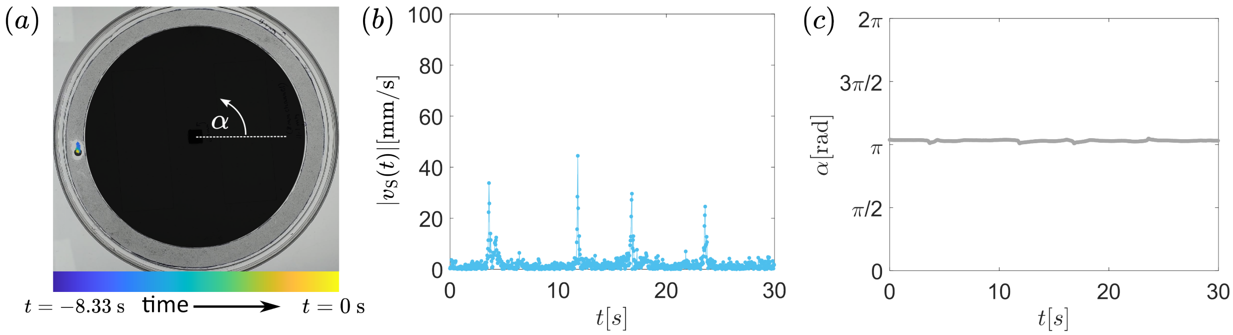


FIG. S4. (a) Representative image of the swimmer along with its trajectory over the last 8.33s for $\phi_{\text{ini}} \approx 0.82$. (b) Temporal evolution of the speed of the swimmer in (a) indicating sporadic instances of motion. (c) Azimuthal position ($\alpha$) of the swimmer in (a).

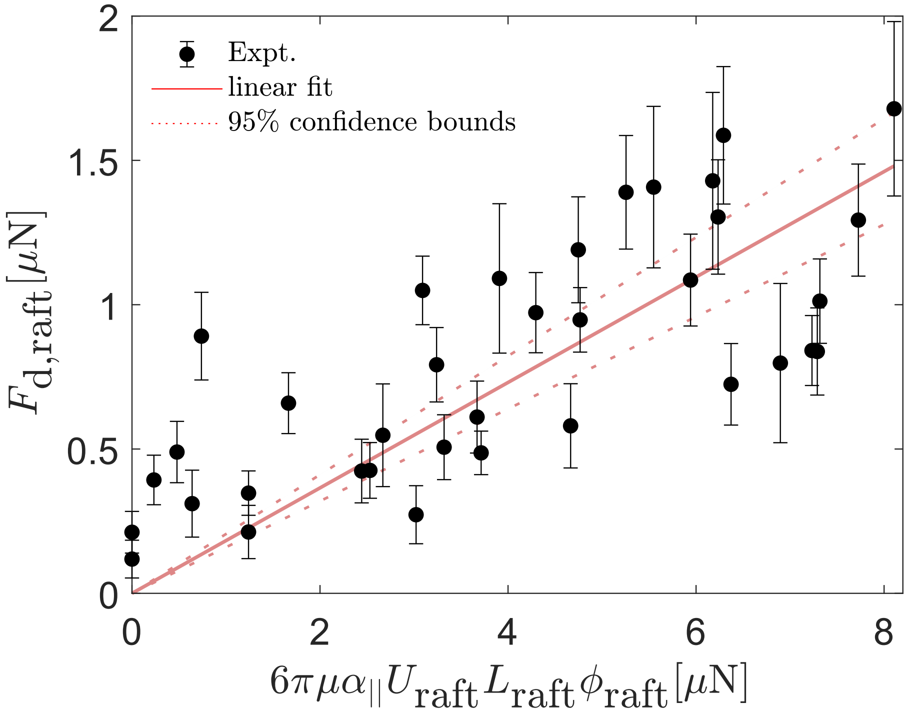


FIG. S5. (a) The linear regression fit of the experimental drag to the model in Eqn. 9, used to estimate the prefactor $K$. The errorbars represent standard deviation.
